# Supplementary material for: I2V: Towards Texture-Aware Self-Supervised Blind Denoising using Self-Residual Learning for Real-World Images
Source: arXiv:2302.10523 source file (2023-02-21)
Supplement: Supplementary file 1 [file macros.tex]

\usepackage{xcolor}
\usepackage{wrapfig}
\usepackage{soul}

\definecolor{yellow}{rgb}{1,1, 0.6}
\definecolor{lightyellow}{rgb}{1,1, 0.8}
\definecolor{orange}{rgb}{1, 0.8, 0.6}
\definecolor{coral}{RGB}{246,131,65}
\definecolor{pinkred}{rgb}{1, 0.6, 0.6}
\definecolor{hotpink}{RGB}{238,64,195}
\definecolor{lavender}{RGB}{207,226,243}
\definecolor{gainsboro}{RGB}{208,224,227}
\definecolor{gainsboro2}{RGB}{217,234,211}
\definecolor{blanchedalmond}{RGB}{252,229,205}

\newcommand{\missfigure}{\textcolor{red}{[F]}}
\newcommand{\misscite}{\textcolor{red}{[C]}}
\newcommand{\missref}{\textcolor{red}{[R]}}

\newcommand{\ray}[1]{{\textcolor{red}{#1}}}
\newcommand{\todo}[1]{{\textcolor{red}{(TODO: #1)}}}

\newcommand{\model}{XXXX}
\newcommand{\modelname}{XXXX\xspace}

\newcommand{\coverage}{spatial coverage\xspace}
\newcommand{\complexity}{detail complexity\xspace}
%altitude or distance
\newcommand{\altitude}{distance\xspace}
\newcommand{\altitudefull}{distance to the scene\xspace}
\newcommand{\altitudes}{distances\xspace}
\newcommand{\altitudesfull}{distances to the scene\xspace}

\newcommand{\copyrightgoogle}{\href{https://www.google.com/help/terms_maps/}{\textcopyright 2022 Google}\xspace}
